# Supplementary material for: femtoPro: Real-time linear and nonlinear optics simulations
Source: arXiv:2503.19627 source file (2025-05-30)
Supplement: Supplementary file 1 [file femtoPro_SI.pdf]

# femtoPro: Real-time linear and nonlinear optics simulations – Supplementary Information

## 1. ELECTRIC FIELD

There are comprehensive books on general optics [1–6] and ultrafast time-resolved spectroscopy [7–15]. Various sign conventions and other conventions exist in the ultrafast optics and spectroscopy literature for which we provide an overview in Table S1. Thus, to avoid inconsistencies, we define all quantities below and furthermore describe the transition between physical electric fields and their algorithmic representation taking into account spatial, spectral–temporal, and amplitude scaling properties in a fashion convenient for real-time simulations.

We start with the real-valued scalar temporal electric field $E(t)$ at a given point in space, including the fast oscillations due to the carrier frequency of visible light. An equivalent, complex-valued, spectral-domain representation is given by

$$E(\omega) = \mathfrak{F}\, E(t) = \frac{1}{\sqrt{2\pi}} \int_{-\infty}^{\infty} E(t) e^{i\omega t}\, \mathrm{d}t \tag{S1}$$

at angular frequency $\omega$, with $\mathfrak{F}$ denoting Fourier transformation, from which the original temporal field can be recovered by inverse Fourier transformation,

$$E(t) = \mathfrak{F}^{-1}\, E(\omega) = \frac{1}{\sqrt{2\pi}} \int_{-\infty}^{\infty} E(\omega) e^{-i\omega t}\, \mathrm{d}\omega. \tag{S2}$$

With $E(t)$ real, it follows that $E(\omega) = E^*(-\omega)$, with the star denoting complex conjugation. Hence, knowledge of the positive-frequency part is sufficient for a full characterization of the light field. We separate [8–11]

$$E(\omega) = \begin{cases} E^+(\omega), & \text{for } \omega \geq 0, \\ E^-(\omega), & \text{for } \omega < 0, \end{cases} \tag{S3}$$

and define $E^+(t)$ as inverse Fourier transform of $E^+(\omega)$,

$$E^+(\omega) = \mathfrak{F}\, E^+(t) \tag{S4}$$

$$= A(\omega) e^{i\Phi(\omega)}, \tag{S5}$$

$$E^+(t) = \mathfrak{F}^{-1}\, E^+(\omega) \tag{S6}$$

$$= A(t) e^{i\Phi(t)}, \tag{S7}$$

with the real-valued quantities named spectral amplitude $A(\omega)$, spectral phase $\Phi(\omega)$, temporal amplitude $A(t)$, and temporal phase $\Phi(t)$. Using the laser center frequency $\omega_0$ that is typically located at the peak of $A(\omega)$ but in principle can be chosen arbitrarily, we introduce the complex temporal envelope

$$\tilde{E}(t) = A(t) e^{i\varphi(t)} \tag{S8}$$

with phase modulation $\varphi(t) = \Phi(t) + \omega_0 t$ such that

$$E^+(t) = \tilde{E}(t) e^{-i\omega_0 t}. \tag{S9}$$

This removes the fast oscillating phase term $\omega_0 t$. The slowly varying phase modulation $\varphi(t)$ describes chirp, i.e., any variation of the oscillation period within the pulse. It is possible to recover the original field $E(t)$ by

$$E(t) = E^+(t) + \text{c.c.} \tag{S10}$$

$$= 2\,\mathrm{Re}\left\{E^+(t)\right\}, \tag{S11}$$

**Table S1.** Overview of common conventions in ultrafast optics and spectroscopy.

| Quantity | Diels [8], Weiner [11] | Wollenhaupt et al. [10] | Trebino [9] |
|---|---|---|---|
| $E(\omega)$ | $\int_{-\infty}^{\infty} E(t)e^{-i\omega t}\,\mathrm{d}t$ | $\int_{-\infty}^{\infty} E(t)e^{-i\omega t}\,\mathrm{d}t$ | $\int_{-\infty}^{\infty} E(t)e^{-i\omega t}\,\mathrm{d}t$ |
| $E(t)$ | $\frac{1}{2\pi}\int_{-\infty}^{\infty} E(\omega)e^{i\omega t}\,\mathrm{d}\omega$ | $\frac{1}{2\pi}\int_{-\infty}^{\infty} E(\omega)e^{i\omega t}\,\mathrm{d}\omega$ | $\frac{1}{2\pi}\int_{-\infty}^{\infty} E(\omega)e^{i\omega t}\,\mathrm{d}\omega$ |
| $E^+(\omega)$ | $A(\omega)e^{i\Phi(\omega)}$ | $A(\omega)e^{-i\Phi(\omega)}$ | $A(\omega)e^{-i\Phi(\omega)}$ |
| $E^+(t)$ | $A(t)e^{i\Phi(t)}$ | $A(t)e^{i\Phi(t)}$ | $A(t)e^{-i\Phi(t)}$ |
| $E^+(\mathbf{r},t)$ | $Ae^{i(\omega_0 t-\mathbf{k}\cdot\mathbf{r})}$ | — | $Ae^{i(\omega_0 t-\mathbf{k}\cdot\mathbf{r})}$ |
| **Quantity** | **Mukamel [7]** | **Yuen-Zhou et al. [15]** | **This work** |
| $E(\omega)$ | $\int_{-\infty}^{\infty} E(t)e^{i\omega t}\,\mathrm{d}t$ | $\int_{-\infty}^{\infty} E(t)e^{i\omega t}\,\mathrm{d}t$ | $\frac{1}{\sqrt{2\pi}}\int_{-\infty}^{\infty} E(t)e^{i\omega t}\,\mathrm{d}t$ |
| $E(t)$ | $\frac{1}{2\pi}\int_{-\infty}^{\infty} E(\omega)e^{-i\omega t}\,\mathrm{d}\omega$ | $\frac{1}{2\pi}\int_{-\infty}^{\infty} E(\omega)e^{-i\omega t}\,\mathrm{d}\omega$ | $\frac{1}{\sqrt{2\pi}}\int_{-\infty}^{\infty} E(\omega)e^{-i\omega t}\,\mathrm{d}\omega$ |
| $E^+(\omega)$ | — | — | $A(\omega)e^{i\Phi(\omega)}$ |
| $E^+(t)$ | — | $\tilde{A}(t)e^{i\Phi_0}$ | $A(t)e^{i\Phi(t)}$ |
| $E^+(\mathbf{r},t)$ | $Ae^{i(\mathbf{k}\cdot\mathbf{r}-\omega_0 t)}$ | $Ae^{i(\mathbf{k}\cdot\mathbf{r}-\omega_0 t)}$ | $Ae^{i(\mathbf{k}\cdot\mathbf{r}-\omega_0 t)}$ |

The long dash "—" indicates that this property is not mentioned explicitly in that source.

where c.c. denotes the complex conjugate of the previous term and is also sometimes called $E^-(t)$ as it is the inverse Fourier transform of $E^-(\omega)$ from Eq. (S3).

The minus sign in Eq. (S9) is a convention frequently employed in the nonlinear spectroscopy community, which is why we also use it here (compare Table S1). Propagating fields with a wave vector $\mathbf{k}$, where $|\mathbf{k}| = 2\pi/\lambda$ at wavelength $\lambda$, are then described by an overall phase factor $e^{i(\mathbf{k}\cdot\mathbf{r}-\omega_0 t)}$ as further explained below. This leads to the conventionally accepted phase-matching directions that signify a rephasing signal along the $-\mathbf{k}_1 + \mathbf{k}_2 + \mathbf{k}_3$ direction, for example, in non-collinear four-wave-mixing spectroscopy. The "disadvantage" of such a choice of the sign convention is that the first-order Taylor coefficient for the spectral phase (see below) does not correspond to the center frequency directly but to its negative. Thus, in the nonlinear optics community one often prefers a convention with $+\omega_0 t$ in Eq. (S9). In that case, the Taylor coefficients do not have an "exceptional" meaning for the frequency, but then the overall phase term $e^{-i(\mathbf{k}\cdot\mathbf{r}-\omega_0 t)}$ requires an additional minus sign, uncustomary in the spectroscopy community. In any event, results for final observables agree with either convention, but one needs to pay attention when comparing intermediate results with the literature.

It is often convenient to express the temporal phase modulation as a Taylor series

$$\Phi(t) = \sum_{j=0}^{\infty} \frac{a_j}{j!} t^j \tag{S12}$$

with Taylor coefficients

$$a_j = \left. \frac{\mathrm{d}^j \Phi(t)}{\mathrm{d}t^j} \right|_{t=0} . \tag{S13}$$

The zero-order coefficient $a_0$ describes the "absolute" or "carrier–envelope" phase, the first-order coefficient is typically taken to define the center frequency via $\omega_0 = -a_1$ (in our sign convention) but can also be used to describe laser pulses with a center frequency different from $\omega_0$ while retaining the general framework of a specified $\omega_0$ in Eq. (S9). Second- and higher-order terms define chirp, i.e., variations of the "momentary frequency"

$$\omega(t) = -\frac{\mathrm{d}\Phi(t)}{\mathrm{d}t} = \omega_0 - \frac{\mathrm{d}\varphi(t)}{\mathrm{d}t}, \tag{S14}$$

where the uncommon minus sign is due to the sign convention of the phase factor we adopted in this work. For example, in the case of "linear chirp," for which only $a_2 \neq 0$ and all higher-order coefficients are equal to zero, $\omega(t)$ varies linearly in time according to $\omega(t) = \omega_0 - a_2 t$ with the "linear-chirp parameter" $a_2$. Analogously, higher Taylor coefficients define higher-order chirp.

Likewise, we may expand the spectral phase into a Taylor series

$$\Phi(\omega) = \sum_{j=0}^{\infty} \frac{b_j}{j!} (\omega - \omega_0)^j \tag{S15}$$

with Taylor coefficients

$$b_j = \left. \frac{\mathrm{d}^j \Phi(\omega)}{\mathrm{d}\omega^j} \right|_{\omega=\omega_0}. \tag{S16}$$

While $b_0 = a_0$ describes a constant phase and $b_1$ a temporal translation of the laser pulse, the coefficients of higher order are responsible for changes in the temporal structure of the electric field. Using a Taylor expansion on either the temporal or the spectral phase (Section 5) or both allows characterization of the electric field with few parameters but comes at the cost of lost generality and, possibly, poor convergence for complicated field profiles.

We define the complex spectral envelope, $\tilde{E}(\omega)$, as Fourier transform of the complex temporal envelope, $\tilde{E}(t)$,

$$\tilde{E}(\omega) = \mathfrak{F}\, \tilde{E}(t), \tag{S17}$$

$$\tilde{E}(t) = \mathfrak{F}^{-1}\, \tilde{E}(\omega), \tag{S18}$$

and determine its relation with $E^{+}(\omega)$ from

$$\tilde{E}(\omega) = \mathfrak{F}\left\{ E^{+}(t) e^{i\omega_0 t} \right\} \tag{S19}$$

$$= \frac{1}{\sqrt{2\pi}} \int_{-\infty}^{\infty} E^{+}(t) e^{i(\omega+\omega_0)t}\, \mathrm{d}t \tag{S20}$$

$$= E^{+}(\omega + \omega_0), \tag{S21}$$

and thus

$$\tilde{E}(\omega - \omega_0) = E^{+}(\omega) \tag{S22}$$

is a frequency-shifted version of $E^{+}(\omega)$.

Let us assume that all quantities above describe a pulse centered around time $t = 0$. Now we add a translation in time by $T$. This may occur, for example, if a pulse propagates by a distance $L$ in vacuum, such that the "propagation time" is given by

$$T = \frac{L}{c} \tag{S23}$$

with $c$ as the velocity of light in vacuum. The case of propagation in media is discussed in Section 4.1 of the main text. In the frequency domain, this propagation corresponds, in principle, to applying a linear spectral phase according to the Fourier-shift theorem and thus a finite parameter $b_1$. Dealing with propagation distances of several meters, it is not practical, however, to apply such a spectral phase modulation to $E^{+}(\omega)$ or $\tilde{E}(\omega)$ directly because only discretely sampled quantities can be stored digitally. Given, for example, a number of $N_\mathrm{s} = 1024$ samples with a sampling step size in time domain of $\delta t \approx 2$ fs to describe short pulses with sufficient resolution, one arrives at a maximum time delay of $N_\mathrm{s}\, \delta t/2 \approx 1$ ps that can be introduced according to the Nyquist sampling theorem, which would correspond to an insufficient maximum spatial distance of $L_\mathrm{max} \approx 0.3$ mm. Thus, instead, we store $T$ of any pulse separately and deal with it only when we have to evaluate the electric field relative to that of another pulse, for example, when describing interference or nonlinear response.

The "propagated" (i.e., time-translated) temporal field is given by

$$E^{+}_{\mathrm{prop}}(t) = E^{+}(t - T) \tag{S24}$$

$$= \tilde{E}(t - T) e^{-i\omega_0 (t-T)} \tag{S25}$$

for propagation time $T$. In frequency domain,

$$E^+_{\text{prop}}(\omega) = \mathfrak{F}\, E^+_{\text{prop}}(t) \tag{S26}$$

$$= \frac{1}{\sqrt{2\pi}} \int_{-\infty}^{\infty} E^+(t-T) e^{i\omega t}\, \mathrm{d}t, \quad \text{substitute } t \to t' = t - T, \tag{S27}$$

$$= \frac{1}{\sqrt{2\pi}} \int_{-\infty}^{\infty} E^+(t') e^{i\omega(t'+T)}\, \mathrm{d}t' \tag{S28}$$

$$= e^{i\omega T} E^+(\omega) \tag{S29}$$

$$= \tilde{E}(\omega - \omega_0) e^{i\omega T}. \tag{S30}$$

Now we take into account the spatial field properties [16], ignoring spatial–temporal couplings that are usually present [17]. The complex-valued Gaussian field dependence for propagation along the $\hat{\mathbf{z}}$ direction can be described by

$$A(r,z) = \frac{w_0}{w(z)} \exp\left[-\frac{r^2}{w^2(z)}\right] e^{i\left[kz + k\frac{r^2}{2R(z)} - \theta(z)\right]} \tag{S31}$$

as a function of radial coordinate $r$ and longitudinal position $z$, beam waist $w_0$, beam radius $w(z)$, wave-vector magnitude $k$, wave-front curvature radius $R(z)$, and Gouy phase $\theta(z) = \arctan(z/z_R)$ that we ignore in the following. The Rayleigh length is defined as

$$z_{\text{R}} = \frac{\pi w_0^2}{\lambda M^2} \tag{S32}$$

with beam-quality factor $M^2$.

We evaluate the spatial evolution of $w(z)$ and $R(z)$ via the complex radius of curvature $q(z)$, given by [16]

$$\frac{1}{q(z)} = \frac{1}{R(z)} + i\frac{\lambda M^2}{\pi w^2(z)}, \tag{S33}$$

and the simple propagation law in free space [18, 19],

$$q(z) = q_0 + z, \tag{S34}$$

as also given in Eq. (66) of the main paper, for propagation by a distance of $z$, where $q_0 = q(0)$.

For normalization of the spatial and time–frequency field components, we note that the "physical," temporal electric field $E(t)$ used above is continuous in $t$ and has units of [V/m]. In an algorithmic representation, we have to store a numerical field that is dimensionless (as it consists of numbers without physical units) and is sampled at discretized times. Electric field strengths may vary over many orders of magnitude depending on the pulse energy, and we want to ensure numerically stable behavior in all cases. Thus we introduce a suitable scaling factor as shown below, such that the sampled numbers are of the order of 1. We begin with the (continuous) momentary power $P(t)$ in [W] that is sampled at discrete times

$$t(j) = t_{\text{min}} + j\,\delta t \tag{S35}$$

throughout the pulse with indices $j = \{0, 1, \ldots, N_{\text{s}} - 1\}$, sampling step size $\delta t$, number of samples $N_{\text{s}}$, and the minimum sampled time point $t_{\text{min}}$. Considering a pulse centered at $t = 0$, we choose

$$t_{\text{min}} = -\frac{N_{\text{s}}\,\delta t}{2} \tag{S36}$$

for symmetry reasons. In the case of propagated pulses [see Eq. (S48) below], we add $T$ to the values of Eq. (S35) when returning the corresponding times. Thus we arrive at the sampled momentary temporal power

$$P_t(j) = P(t(j)) \tag{S37}$$

with $t(j)$ from Eq. (S35).

The pulse energy $W$ in [J] is then given by

$$W = \int_{-\infty}^{\infty} P(t)\, \mathrm{d}t \tag{S38}$$

$$\approx \sum_{j=0}^{N_{\text{s}}-1} P_t(j)\, \delta t. \tag{S39}$$

We introduce the pulse-energy scaling factor $S$ such that

$$W = SE^2 \tag{S40}$$

with $E$ signifying the Euclidian (or $L^2$) norm of $\tilde{E}(t)$, i.e.,

$$E = \sqrt{\sum_{j=0}^{N_s-1} \left|\tilde{E}_t(j)\right|^2}, \tag{S41}$$

where $\tilde{E}_t(j)$, in the computational framework, is the dimensionless array of the complex temporal envelope, and the squaring of the norm $E$ in Eq. (S40) arises because we need to sum up the temporal intensities, without taking the square root afterwards. Whenever $\tilde{E}_t(j)$ is accessed in memory for a requested time $t$, one selects the element $j$ for which $t = t(j)$, with $t(j)$ given in Eq. (S35).

We define an initial value of $S$, named $S_0$, using an initial pulse energy $W_0$, by setting

$$S_0 = W_0 \quad \text{and} \quad E_0 = 1, \tag{S42}$$

where the latter condition is reached through appropriate initial normalization of $\tilde{E}_t(j)$, see Eq. (S47) below. Manipulating the energy of a laser beam can then be carried out either by changing $S$ directly or by changing $\tilde{E}_t(j)$. The former is useful, e.g., when implementing simple optical elements with non-unity transmission or reflection, while the latter is useful, e.g., in nonlinear optics and spectroscopy where signal fields arise from appropriate multiplication of input fields. If the numbers stored in $\tilde{E}_t(j)$ get too small and lead to numerical artifacts, appropriate rescaling with a factor of $F$ is possible if $S$ is rescaled simultaneously by $1/F^2$.

Using the discretized, dimensionless, complex time envelope, we get the momentary temporal power in correct physical units via

$$P_t(j) = \frac{S}{\delta t} \left|\tilde{E}_t(j)\right|^2. \tag{S43}$$

Taking into account the spatial property with a beam radius of $w(z)$, this corresponds to an intensity in [W/m$^2$] of

$$I_t(j) = \frac{2P_t(j)}{\pi w^2(z)} \tag{S44}$$

on the center axis of the beam [from Eq. (S91) for identical beams], which corresponds to twice the intensity averaged over the full cross section.

Note that, conventionally, the temporal intensity of a pulse is defined within the slowly-varying envelope approximation as

$$I(t) = 2\varepsilon_0 c n A^2(t), \tag{S45}$$

wherein $\varepsilon_0$ is the vacuum permittivity, $c$ the vacuum velocity of light, and $n$ the refractive index of the medium in which the intensity is measured. The temporal intensity averages over the individual carrier-frequency oscillations of the electric field but retains the overall shape due to the envelope. For this definition, $A(t)$ has to be provided in the correct physical units of electric field strength in [V/m], whereas we have chosen to work with the more directly accessible pulse energy as a scaling factor.

We define pulse duration $\tau_\mathrm{p}$ as the full width at half maximum (FWHM) of the spectral power density, which is appropriate for simple envelopes. The duration of more complex pulse shapes may be better characterized with second-order moments [8] or rather the full field profile directly. Thus, we use pulse duration mainly to define initial pulses emitted from a laser via

$$\tilde{E}_{t,\text{non-normalized}}(j) = \exp\left[-(2\ln 2)\,\frac{t^2(j)}{\tau_\mathrm{p}^2}\right], \tag{S46}$$

$$\tilde{E}_t(j) = \frac{\tilde{E}_{t,\text{non-normalized}}(j)}{\sqrt{\sum_{j=0}^{N_s-1}\left|\tilde{E}_{t,\text{non-normalized}}(j)\right|^2}}, \tag{S47}$$

with $t(j)$ from Eq. (S35), where $\tilde{E}_t(j)$ fulfills the norm $E = 1$ from Eq. (S41).

Combining spatial and temporal properties and allowing the beam to be displaced in the transverse $\hat{\mathbf{x}}$ and $\hat{\mathbf{y}}$ directions by $x_0$ and $y_0$, respectively, we define the temporally propagated

spatial–temporal field under the scaling conditions of Eqs. (S38)–(S43) and combining Eq. (S25) and Eq. (S31), noting that we approximate $R \to \infty$ and $\theta = 0$, as

$$E^{+}_{\text{prop}}(x, y, z, t) = \sqrt{\frac{2}{\pi}} \frac{1}{w(z)} \exp\left[-\frac{(x - x_0)^2 + (y - y_0)^2}{w^2(z)}\right] e^{i\mathbf{k}\cdot\mathbf{r}} \sqrt{\frac{S}{\delta t}} \tilde{E}_t(j) e^{-i\omega_0(t-T)}, \tag{S48}$$

from which we obtain the momentary temporal power by spatial integration of the absolute magnitude squared,

$$P_t(j) = \int_{-\infty}^{\infty} \int_{-\infty}^{\infty} \left| E^{+}_{\text{prop}}(x, y, z, t) \right|^2 \, \mathrm{d}x \, \mathrm{d}y. \tag{S49}$$

Note that, due to our choice of normalization, the proportionality factor of Eq. (S45) is not present in Eq. (S49).

In complete analogy, we define the corresponding quantities in frequency domain, starting with the spectral power $P(\omega)$, noting, however, that it is not measured in [W] as the temporal power but rather in [J/(rad s$^{-1}$)], i.e., energy per angular frequency sampling step. It is sampled at discrete angular frequencies

$$\omega(j) = \omega_{\text{min}} + j \, \delta\omega \tag{S50}$$

with indices $j = \{0, 1, \ldots, N_\text{s} - 1\}$, frequency sampling step size

$$\delta\omega = \frac{2\pi}{N_\text{s} \, \delta t} \tag{S51}$$

due to Fourier-transformation properties, number of samples $N_\text{s}$ equal to the number of samples in the time domain, and minimum sampled frequency

$$\omega_{\text{min}} = -\frac{N_\text{s} \, \delta\omega}{2} = -\frac{\pi}{\delta t}. \tag{S52}$$

Similar to the case of the temporal field, we add $\omega_0$ to the values in Eq. (S50) for retrieving the "physical" quantities, according to Eq. (S30). In that case, the situation may arise that $\omega_0 < |\omega_{\text{min}}|$ if the temporal sampling step is chosen as $\delta t < \pi/\omega_0$, i.e., if more than two samples are taken per carrier oscillation period. This results in negative "physical" frequencies $\omega(j) + \omega_0$. We have already seen that such negative frequencies arise naturally after Fourier transformation for $E(\omega)$ in Eq. (S1). Here, however, we deal with $E^{+}(\omega)$ from Eq. (S3) that is zero for negative frequencies. Thus, any sampled values should be zero for such frequencies. In practice, when displaying physical properties for such negative frequencies, they are thus ignored. However, we point out that the separation in Eq. (S3) is problematic for pulses with an extremely broad spectrum, i.e., if the spectral bandwidth approaches $\omega_0$, because then they will not have decayed when approaching zero frequency, and then the simple separation into $E^{+}(\omega)$ and $E^{-}(\omega)$ with according symmetry properties does not hold. For pulses with an extremely broad spectrum, one would anyway need more than two sampling points per oscillation period (as defined for the center frequency) to describe the field because for frequencies much larger than the center frequency, the field oscillates faster. This is consistent with the limit derived above. Then the slowly varying envelope approximation breaks down. In the present work, we always remain within this approximation, however, for computational reasons, which is a limitation one should be aware of. In that case, negative frequencies for $E^{+}(\omega)$ are not required and we can choose $\delta t \geq \pi/\omega_0$. One might select $\delta t = \pi/\omega_0$ for maximal spectral coverage. However, in order to realize sufficient computational speed, one also has to keep the number of samples $N_\text{s}$ small enough for all array operations. This, in turn, reduces the maximum treatable time range that is given by $N_\text{s} \, \delta t$ according to Eq. (S36), so that one might wish to seek a compromise for both $N_\text{s}$ and $\delta t$.

Using the definition for the sampling grid, we obtain the sampled spectral power

$$P_\omega(j) = P(\omega(j)) \tag{S53}$$

with $\omega(j)$ from Eq. (S50) and the pulse energy $W$ in [J] by

$$W = \int_{-\infty}^{\infty} P(\omega) \, \mathrm{d}\omega \tag{S54}$$

$$\approx \sum_{j=0}^{N_\text{s}-1} P_\omega(j) \, \delta\omega. \tag{S55}$$

Using the same pulse-energy scaling factor $S$ as above, we get the spectral power via

$$P_\omega(j) = \frac{S}{\delta\omega} \left|\tilde{E}_\omega(j)\right|^2 \tag{S56}$$

and the spectral intensity

$$I_\omega(j) = \frac{2P_\omega(j)}{\pi w^2(z)} \tag{S57}$$

on the center axis of the beam, which corresponds to twice the spectral intensity averaged over the full cross section.

Note that $\tilde{E}_\omega(j)$ and $\tilde{E}_t(j)$ form a Fourier pair,

$$\tilde{E}_\omega(j) = \mathfrak{F}_{\text{discrete}}\, \tilde{E}_t(j), \tag{S58}$$

$$\tilde{E}_t(j) = \mathfrak{F}^{-1}_{\text{discrete}}\, \tilde{E}_\omega(j), \tag{S59}$$

where $\mathfrak{F}_{\text{discrete}}$ indicates a discrete version of the Fourier transformation, in our case implemented as a "Fast Fourier Transformation" (FFT) algorithm, ensuring that the number of samples, $N_s$, is defined as a power of 2. In the algorithmic implementation, the inter-conversion between the two quantities is automatically carried out only when necessary.

We obtain the temporally propagated spatial–spectral field considering Eq. (S30),

$$E^+_{\text{prop}}(x, y, z, \omega) = \sqrt{\frac{2}{\pi}} \frac{1}{w(z)} \exp\left[-\frac{(x-x_0)^2 + (y-y_0)^2}{w^2(z)}\right] e^{i\mathbf{k}\cdot\mathbf{r}} \sqrt{\frac{S}{\delta\omega}} \tilde{E}_\omega(j) e^{i\omega T}, \tag{S60}$$

from which we obtain the spectral power by spatial integration of the absolute magnitude squared,

$$P_\omega(j) = \int_{-\infty}^{\infty} \int_{-\infty}^{\infty} \left|E^+_{\text{prop}}(x, y, z, \omega)\right|^2 \mathrm{d}x\,\mathrm{d}y. \tag{S61}$$

Note that we treat the electric field as a scalar throughout. Conceptually, it is not difficult to incorporate polarization phenomena by treating the electric field as a vector.

## 2. OVERLAP OF TWO-DIMENSIONAL GAUSSIAN FUNCTIONS

While in Section 3.1 of the main paper we considered the geometric overlap of a laser beam with a hard aperture, we now investigate the overlap of two laser-beam cross sections, but only in the limit of normal incidence, which will be relevant for calculations of interference between several beams and for nonlinear signal generation. Thus we determine the product of two two-dimensional Gaussian distributions,

$$A_k(x, y) = A_k e^{-\alpha_k(x-x_k)^2 - \beta_k(y-y_k)^2}, \quad k = \{1, 2\}, \tag{S62}$$

centered at $(x_k, y_k)$ and characterized by (potentially different) width parameters,

$$\alpha_k = \frac{1}{w^2_{k,x}}, \quad \beta_k = \frac{1}{w^2_{k,y}}, \tag{S63}$$

along the $\hat{\mathbf{x}}$ and $\hat{\mathbf{y}}$ directions, respectively. The product is

$$A_p(x, y) = A_1(x, y) A_2(x, y) \tag{S64}$$

$$= A_1 A_2 e^{-[\alpha_1(x-x_1)^2 + \alpha_2(x-x_2)^2]} e^{-[\beta_1(y-y_1)^2 + \beta_2(y-y_2)^2]}. \tag{S65}$$

We hypothesize that $A_p(x, y)$ can be written in the form of a new Gaussian with parameters to be determined. For this purpose, we modify the exponent of the first exponential term by

multiplying out the binomial terms and "completing the squares,"

$$\alpha_1(x-x_1)^2+\alpha_2(x-x_2)^2 \tag{S66}$$

$$=(\alpha_1+\alpha_2)x^2-2(\alpha_1x_1+\alpha_2x_2)x+\alpha_1x_1^2+\alpha_2x_2^2 \tag{S67}$$

$$=(\alpha_1+\alpha_2)\left(x^2-2\frac{\alpha_1x_1+\alpha_2x_2}{\alpha_1+\alpha_2}x+\frac{\alpha_1x_1^2+\alpha_2x_2^2}{\alpha_1+\alpha_2}\right) \tag{S68}$$

$$=(\alpha_1+\alpha_2)\left[\left(x-\frac{\alpha_1x_1+\alpha_2x_2}{\alpha_1+\alpha_2}\right)^2+\frac{\alpha_1x_1^2+\alpha_2x_2^2}{\alpha_1+\alpha_2}-\frac{(\alpha_1x_1+\alpha_2x_2)^2}{(\alpha_1+\alpha_2)^2}\right] \tag{S69}$$

$$=(\alpha_1+\alpha_2)\left[\left(x-\frac{\alpha_1x_1+\alpha_2x_2}{\alpha_1+\alpha_2}\right)^2+\frac{(\alpha_1+\alpha_2)(\alpha_1x_1^2+\alpha_2x_2^2)-(\alpha_1x_1+\alpha_2x_2)}{(\alpha_1+\alpha_2)^2}\right] \tag{S70}$$

$$=(\alpha_1+\alpha_2)\left[\left(x-\frac{\alpha_1x_1+\alpha_2x_2}{\alpha_1+\alpha_2}\right)^2+\frac{\alpha_1\alpha_2}{(\alpha_1+\alpha_2)^2}(x_1-x_2)^2\right] \tag{S71}$$

$$=(\alpha_1+\alpha_2)\left(x-\frac{\alpha_1x_1+\alpha_2x_2}{\alpha_1+\alpha_2}\right)^2+\frac{\alpha_1\alpha_2}{\alpha_1+\alpha_2}(x_1-x_2)^2. \tag{S72}$$

Using the analogous strategy for the second exponential term with the $y$ coordinates, we find the product to be another Gaussian as hypothesized,

$$A_{\text{p}}(x,y)=A_{\text{p}}e^{-\alpha_{\text{p}}(x-x_{\text{p}})^2-\beta_{\text{p}}(y-y_{\text{p}})^2}, \tag{S73}$$

with product width parameters

$$\alpha_{\text{p}}=\alpha_1+\alpha_2,\quad \beta_{\text{p}}=\beta_1+\beta_2, \tag{S74}$$

center position

$$x_{\text{p}}=\frac{\alpha_1x_1+\alpha_2x_2}{\alpha_1+\alpha_2},\quad y_{\text{p}}=\frac{\beta_1y_1+\beta_2y_2}{\beta_1+\beta_2}, \tag{S75}$$

and amplitude

$$A_{\text{p}}=A_1A_2\exp\left[-\frac{\alpha_1\alpha_2}{\alpha_1+\alpha_2}(x_1-x_2)^2\right]\exp\left[-\frac{\beta_1\beta_2}{\beta_1+\beta_2}(y_1-y_2)^2\right]. \tag{S76}$$

Using the notation with beam radii, this corresponds to a Gaussian

$$A_{\text{p}}(x,y)=A_{\text{p}}\exp\left[-\frac{(x-x_{\text{p}})^2}{w_{\text{p},x}^2}-\frac{(y-y_{\text{p}})^2}{w_{\text{p},y}^2}\right], \tag{S77}$$

centered at

$$x_{\text{p}}=\frac{\frac{x_1}{w_{1,x}^2}+\frac{x_2}{w_{2,x}^2}}{\frac{1}{w_{1,x}^2}+\frac{1}{w_{2,x}^2}},\quad y_{\text{p}}=\frac{\frac{y_1}{w_{1,y}^2}+\frac{y_2}{w_{2,y}^2}}{\frac{1}{w_{1,y}^2}+\frac{1}{w_{2,y}^2}}, \tag{S78}$$

with radii

$$w_{\text{p},x}=\frac{1}{\sqrt{\frac{1}{w_{1,x}^2}+\frac{1}{w_{2,x}^2}}},\quad w_{\text{p},y}=\frac{1}{\sqrt{\frac{1}{w_{1,y}^2}+\frac{1}{w_{2,y}^2}}} \tag{S79}$$

along the $\hat{\mathbf{x}}$ and $\hat{\mathbf{y}}$ directions, respectively, and a product amplitude of

$$A_{\text{p}}=A_1A_2\exp\left[-\frac{(x_1-x_2)^2}{w_{1,x}^2+w_{2,x}^2}-\frac{(y_1-y_2)^2}{w_{1,y}^2+w_{2,y}^2}\right]. \tag{S80}$$

We now determine the field overlap integral $W_{\text{p}}$ that is relevant for the scaling of linear interference fringes and nonlinear signal generation. Due to the Gaussian function, the integration can be carried out analytically and delivers

$$W_{\text{p}}=\int_{-\infty}^{\infty}\int_{-\infty}^{\infty}A_{\text{p}}(x,y)\,\mathrm{d}x\,\mathrm{d}y \tag{S81}$$

$$=A_{\text{p}}\int_{-\infty}^{\infty}e^{-\alpha_{\text{p}}(x-x_{\text{p}})^2}\,\mathrm{d}x\int_{-\infty}^{\infty}e^{-\beta_{\text{p}}(y-y_{\text{p}})^2}\,\mathrm{d}y \tag{S82}$$

$$=A_{\text{p}}\sqrt{\frac{\pi}{\alpha_{\text{p}}}}\sqrt{\frac{\pi}{\beta_{\text{p}}}}. \tag{S83}$$

For further simplification, we consider circularly symmetric Gaussians (i.e., stigmatic beams as assumed in the main text) with $\alpha_j = \beta_j$. In that case, the width parameters in Eq. (S76) simplify to

$$\frac{\alpha_1\alpha_2}{\alpha_1+\alpha_2} = \frac{\beta_1\beta_2}{\beta_1+\beta_2} \tag{S84}$$

$$= \frac{\frac{1}{w_1^2}\frac{1}{w_2^2}}{\frac{1}{w_1^2}+\frac{1}{w_2^2}} \tag{S85}$$

$$= \frac{1}{w_1^2+w_2^2}, \tag{S86}$$

and thus

$$A_\mathrm{p} = A_1 A_2 \exp\left[-\frac{(x_1-x_2)^2+(y_1-y_2)^2}{w_1^2+w_2^2}\right]. \tag{S87}$$

The overlap integral in Eq. (S83), for circularly symmetric Gaussians, simplifies to

$$W_\mathrm{p} = A_\mathrm{p}\sqrt{\frac{\pi}{\alpha_1+\alpha_2}}\sqrt{\frac{\pi}{\beta_1+\beta_2}} \tag{S88}$$

$$= A_\mathrm{p}\frac{\pi}{\sqrt{\left(\frac{1}{w_1^2}+\frac{1}{w_2^2}\right)\left(\frac{1}{w_1^2}+\frac{1}{w_2^2}\right)}} \tag{S89}$$

$$= A_\mathrm{p}\frac{\pi}{\frac{1}{w_1^2}+\frac{1}{w_2^2}} \tag{S90}$$

$$= A_1 A_2 \frac{\pi}{\frac{1}{w_1^2}+\frac{1}{w_2^2}}\exp\left[-\frac{(x_1-x_2)^2+(y_1-y_2)^2}{w_1^2+w_2^2}\right]. \tag{S91}$$

For determining the overlap between three Gaussians, $A_1(x,y)$, $A_2(x,y)$, and $A_3(x,y)$, we obtain first the overlap between, say, $A_2(x,y)$ and $A_3(x,y)$, according to the procedure above, and then repeat the calculation a second time replacing $A_2$ with $A_\mathrm{p}$ from the first step, $(x_2, y_2)$ with $(x_\mathrm{p}, y_\mathrm{p})$ from the first step, and $w_2$ with $w_\mathrm{p}$ from the first step. Analogously, this can be extended to more than three Gaussians. The order of calculation in this algorithm is irrelevant because each calculation step delivers a Gaussian again, and the multiplications are commutative and associative.

## 3. GAUSSIAN TRANSMISSION THROUGH A CIRCULAR APERTURE

We determine the relative transmission factor of a Gaussian laser beam through a circular aperture numerically. Without loss of generality, we assume that the incident beam is displaced by $d$ (compare Fig. 1 of the main text) along the $\hat{\mathbf{x}}$ axis with respect to the center of the GOE aperture. Using Eqs. (S57), (S60) and (S61), the transverse beam intensity is given by

$$I(x,y) = I_0 \exp\left[-2\frac{(x-x_0)^2+(y-y_0)^2}{w^2}\right] \tag{S92}$$

with the on-axis intensity $I_0$ and, in our case, $x_0 = d$ and $y_0 = 0$. For normalization, the full power of the incident beam,

$$P_\mathrm{in} = \int_{-\infty}^{\infty} \mathrm{d}x \int_{-\infty}^{\infty} \mathrm{d}y\, I(x,y), \tag{S93}$$

is obtained with help of Eq. (S57) as

$$P_\mathrm{in} = I_0 \frac{\pi w^2}{2}. \tag{S94}$$

The outgoing, potentially clipped, beam power is obtained, instead, by restricting the integration area to the circular aperture,

$$P_\mathrm{out} = I_0 \int_{(x^2+y^2\le a^2)} \mathrm{d}x \int \mathrm{d}y\, \exp\left[-2\frac{(x-d)^2}{w^2} - 2\frac{y^2}{w^2}\right]. \tag{S95}$$

It is convenient to express all spatial quantities in units of the beam radius $w$ because only the ratios determine transmission. Then, we substitute

$$x \quad \rightarrow \quad x' = \frac{x}{w}, \quad \mathrm{d}x = w\,\mathrm{d}x', \tag{S96}$$

$$y \quad \rightarrow \quad y' = \frac{y}{w}, \quad \mathrm{d}y = w\,\mathrm{d}y', \tag{S97}$$

$$a \quad \rightarrow \quad a' = \frac{a}{w}, \tag{S98}$$

$$d \quad \rightarrow \quad d' = \frac{d}{w}, \tag{S99}$$

$$\tag{S100}$$

to get

$$P_{\mathrm{out}} = I_0 w^2 \int\limits_{(x'^2+y'^2 \leq a'^2)} \mathrm{d}x' \int \mathrm{d}y'\, e^{-2[(x'-d')^2 - y'^2]}. \tag{S101}$$

The integral is symmetric in $y'$, providing a factor of 2 below, and we can insert explicit expressions for the integral limits,

$$P_{\mathrm{out}} = 2I_0 w^2 \int_{-a'}^{a'} \mathrm{d}x' \int_0^{\sqrt{a'^2 - x'^2}} \mathrm{d}y'\, e^{-2[(x'-d')^2 - y'^2]}, \tag{S102}$$

from which we proceed, for numerical evaluation, by discretizing

$$\mathrm{d}x' \quad \rightarrow \quad \Delta x' = \frac{2a'}{N}, \tag{S103}$$

$$\mathrm{d}y' \quad \rightarrow \quad \Delta y' = \frac{2a'}{N}, \tag{S104}$$

for a number of $N$ samples for $x'$ from $-a'$ to $a'$, and employing the same resolution for $y'$. Thus, using integer indices $i$ and $j$, we have to evaluate the intensity at coordinates

$$x' = -a' + (i + \frac{1}{2})\Delta x', \quad i = 0, \ldots, N-1, \tag{S105}$$

$$y' = (j + \frac{1}{2})\Delta y', \quad j = 0, \ldots, j_{\max}, \tag{S106}$$

with the maximum index along the $y$ coordinate obtained from the integral limit $y'_{\max} = \sqrt{a'^2 - x'^2}$ as

$$j_{\max} = \left\lfloor \frac{y'_{\max}}{\Delta y'} \right\rfloor = \left\lfloor \frac{N}{2}\sqrt{1 - \frac{x'^2}{a'^2}} \right\rfloor \tag{S107}$$

with the "floor" operator $\lfloor\rfloor$ that provides the greatest integer less than or equal to its argument. Thus we can replace the integrals with discrete sums and obtain the transmission factor

$$T = \frac{P_{\mathrm{out}}}{P_{\mathrm{in}}} \tag{S108}$$

from evaluating

$$T = \frac{16a'^2}{\pi N^2} \sum_{i=0}^{N-1} \sum_{j=0}^{j_{\max}} e^{-2[(x'-d')^2 - y'^2]}. \tag{S109}$$

We precalculate $T(a', d')$ for a two-dimensional set of $a'$ and $d'$ and then simply have to read off the appropriate result during real-time evaluation. In order to obtain a sufficiently large resolution of the $T$ matrix, we use a size of 500 by 500 grid points with aperture and shift step sizes of $\Delta a' = 0.010w$ and $\Delta d' = 0.012w$, respectively. Transmission factor values between grid points are obtained by rounding the fractional indices $a'/\Delta a'$ and $d'/\Delta d'$ to the indices of the nearest grid point.

In case of large circular apertures relative to the beam radius, i.e., $a \gg w$, the beam clipping can be approximated as clipping at a straight edge. We set the boundary above which this

approximation takes place to $a = 5w$. The outgoing power of the clipped beam is then obtained by setting the lower integration bound along $x$ to $a$, leading to

$$P_{\text{out}} = \int_a^\infty \mathrm{d}x \int_{-\infty}^\infty \mathrm{d}y \, I(x,y), \tag{S110}$$

which can further be expressed using Eqs. Eq. (S92), Eq. (S93), and Eq. (S94) as

$$P_{\text{out}} = I_0 \sqrt{\frac{\pi w^2}{2}} \int_a^\infty \mathrm{d}x \exp\left[-2\frac{(x-d)^2}{w^2}\right]. \tag{S111}$$

The integral in Eq. (S111) can be solved by substituting

$$x \to x' = x - d, \quad \mathrm{d}x = \mathrm{d}x', \tag{S112}$$

which results in

$$P_{\text{out}} = I_0 \sqrt{\frac{\pi w^2}{2}} \int_{a-d}^\infty \mathrm{d}x' \exp\left[-2\frac{x'^2}{w^2}\right], \tag{S113}$$

where we further substitute

$$x' \to t = \frac{\sqrt{2}}{w} x', \quad \mathrm{d}x' = \frac{w}{\sqrt{2}} \mathrm{d}t, \tag{S114}$$

to obtain

$$P_{\text{out}} = I_0 \frac{\sqrt{\pi}}{2} w^2 \int_{\frac{\sqrt{2}}{w}(a-d)}^\infty \mathrm{d}t \, e^{-t^2}. \tag{S115}$$

Using the definition of the complementary error function,

$$\operatorname{erfc} x = \frac{2}{\sqrt{\pi}} \int_x^\infty \mathrm{d}t \, e^{-t^2}, \tag{S116}$$

Eq. (S115) can be rewritten as

$$P_{\text{out}} = I_0 \frac{\pi}{4} w^2 \operatorname{erfc}\left[\frac{\sqrt{2}}{w}(a-d)\right]. \tag{S117}$$

The transmission factor in case of clipping at a straight edge is thus given by

$$T = \frac{P_{\text{out}}}{P_{\text{in}}} = \frac{1}{2} \operatorname{erfc}\left[\sqrt{2}(a'-d')\right], \tag{S118}$$

where aperture radius and displacement are expressed in units of the beam radius $w$, i.e., $a' = a/w$ and $d' = d/w$, respectively.

## 4. INTERFERENCE VISIBILITY FACTOR

We solve Eq. (27) from the main text by substituting $x \to \tilde{x} = x - x_{\text{p}}$ and $y \to \tilde{y} = y - y_{\text{p}}$ to make the integrals symmetric around the origin, pulling out all factors that are independent of $\tilde{x}$ and $\tilde{y}$, and separating the $\tilde{x}$ and $\tilde{y}$ integrals,

$$\begin{aligned}\eta_{k,l} = \frac{2}{\pi w_k w_l} \exp\left[-\frac{(x_k - x_l)^2 + (y_k - y_l)^2}{w_k^2 + w_l^2}\right] e^{i(\Delta k_x x_{\text{p}} + \Delta k_y y_{\text{p}})} \\ \times \int_{-\infty}^\infty \exp\left[-\left(\frac{1}{w_k^2} + \frac{1}{w_l^2}\right)\tilde{x}^2\right] e^{i\Delta k_x \tilde{x}} \, \mathrm{d}\tilde{x} \int_{-\infty}^\infty \exp\left[-\left(\frac{1}{w_k^2} + \frac{1}{w_l^2}\right)\tilde{y}^2\right] e^{i\Delta k_y \tilde{y}} \, \mathrm{d}\tilde{y}.\end{aligned} \tag{S119}$$

Consider the first of the remaining two integrals and write the complex exponential using Euler's formula,

$$\begin{aligned}\int_{-\infty}^\infty \exp\left[-\left(\frac{1}{w_k^2} + \frac{1}{w_l^2}\right)\tilde{x}^2\right] e^{i\Delta k_x \tilde{x}} \, \mathrm{d}\tilde{x} = \int_{-\infty}^\infty \exp\left[-\left(\frac{1}{w_k^2} + \frac{1}{w_l^2}\right)\tilde{x}^2\right] \cos(\Delta k_x \tilde{x}) \, \mathrm{d}\tilde{x} \\ + i \int_{-\infty}^\infty \exp\left[-\left(\frac{1}{w_k^2} + \frac{1}{w_l^2}\right)\tilde{x}^2\right] \sin(\Delta k_x \tilde{x}) \, \mathrm{d}\tilde{x},\end{aligned} \tag{S120}$$

then the second term disappears for symmetry reasons and the remaining Gaussian integral evaluates to

$$\int_{-\infty}^{\infty} \exp\left[-\left(\frac{1}{w_k^2}+\frac{1}{w_l^2}\right)\tilde{x}^2\right]\cos(\Delta k_x \tilde{x})\,\mathrm{d}\tilde{x} = \sqrt{\frac{\pi}{\frac{1}{w_k^2}+\frac{1}{w_l^2}}}\exp\left[-\frac{\Delta k_x^2}{4\left(\frac{1}{w_k^2}+\frac{1}{w_l^2}\right)}\right]. \tag{S121}$$

The second integral in Eq. (S119) evaluates analogously, delivering

$$\eta_{k,l} = \frac{2}{\pi w_k w_l}\frac{\pi}{\frac{1}{w_k^2}+\frac{1}{w_l^2}}\exp\left[-\frac{(x_k-x_l)^2+(y_k-y_l)^2}{w_k^2+w_l^2}\right]e^{i(\Delta k_x x_\mathrm{p}+\Delta k_y y_\mathrm{p})}\exp\left[-\frac{\Delta k_x^2+\Delta k_y^2}{2\left(\frac{1}{w_k^2}+\frac{1}{w_l^2}\right)}\right] \tag{S122}$$

$$= \frac{2W_\mathrm{p}}{\pi w_k w_l}e^{i(\Delta k_x x_\mathrm{p}+\Delta k_y y_\mathrm{p})}\exp\left[-\frac{\Delta k_x^2+\Delta k_y^2}{2\left(\frac{1}{w_k^2}+\frac{1}{w_l^2}\right)}\right] \tag{S123}$$

using $W_\mathrm{p}$ from Eq. (S91) with $A_1 = A_2 = 1$, representing the overlap area, and thus yields Eq. (28) from the main text.

In the limiting case of identical beam radii $w = w_k = w_l$ and identical intersection positions $(x_k, y_k) = (x_l, y_l)$ but different incidence directions, one finds $W_\mathrm{p} = \pi w^2/2$ and

$$\eta_{k,l} = \exp\left[-\frac{w^2(\Delta k_x^2+\Delta k_y^2)}{4}\right]. \tag{S124}$$

In another limiting case of Eq. (S123), considering identical directions but displaced beams, one finds

$$\eta_{k,l} = \frac{2W_\mathrm{p}}{\pi w_k w_l} \tag{S125}$$

such that visibility is determined by the overlap area, i.e., for beams with less mutual overlap, the interference visibility is decreased as expected. Finally, if all parameters are identical, $\eta_{k,l} = 1$ leads to perfect visibility.

We can use this result to estimate the degree of alignment accuracy required for the observation of spectral interference. If we require a visibility of at least $\eta_{k,l} = 1/e = 37$ %, this corresponds to a radial (transverse) wave-vector mismatch (equal to the total wave-vector mismatch at identical carrier frequencies) of at most

$$\Delta k_r = \sqrt{\Delta k_x^2+\Delta k_y^2} = \frac{2}{w} \tag{S126}$$

in the limit of Eq. (S124), corresponding to an angular mismatch of

$$\Delta\alpha = \frac{\Delta k_r}{k} = \frac{\lambda}{\pi w} \tag{S127}$$

for the common beam radius $w$. At a propagation length $L$, the initial lateral displacement thus may be at maximum

$$\Delta r = \Delta\alpha\, L = \frac{\lambda L}{\pi w}. \tag{S128}$$

Inserting typical values of $\lambda = 800$ nm, $L = 0.5$ m and $w = 1$ mm, one obtains $\Delta r = 0.1$ mm, which explains why micrometer fine-adjustment screws are helpful to align an interferometer. If we consider the minimal possible beam radius $w_\mathrm{min}$ from Eq. (S147) in a tight focus, we obtain a comparatively large allowed angular difference of $\Delta\alpha = 1/M^2 = 1$ rad for a Gaussian beam from Eq. (S127), which makes sense intuitively because for a diffraction-limited spot, all partial wavelets with different beam directions add up constructively.

In the literature, the deduction in the previous paragraph is formulated to indicate that there is no phase mismatch in the focus of a microscope. This is relevant for nonlinear spectroscopy that uses phase matching to distinguish signal contributions and is thus not applicable in a very tight focus. Instead, phase matching for nonlinear spectroscopy works rather in the opposite limit of plane waves. In the context of spectral interference visibility, this finding means that focusing the beams improves the visibility contrast for a given angular mismatch. Likewise, visibility

can be improved, with indirect proportionality according to Eq. (S128), by closing an entrance aperture $a$ directly in front of the spectrometer (thus decreasing $w = a$). This is because selecting a small region from the spatial interference pattern – ideally containing only one interference fringe within the aperture – results in maximum contrast.

Concerning transverse displacement at the detector position, one obtains, for identical beam radii and identical directions,

$$\eta_{k,l} = \exp\left[-\frac{(x_1 - x_2)^2 + (y_1 - y_2)^2}{2w^2}\right] \tag{S129}$$

from Eq. (S125) and Eq. (S91). Requiring again $\eta_{k,l} = 1/e$, this leads to a maximally allowed beam displacement of

$$\Delta r = \sqrt{\Delta x^2 + \Delta y^2} = \sqrt{2}\, w, \tag{S130}$$

and thus $\Delta r = 1.4$ mm for the same exemplary beam radius of $w = 1$ mm.

Hence, for these parameters, lateral parallel displacement is somewhat more "forgiving" compared to angular mismatch arising from the same amount of lateral displacement (but then overlapping beams at the intersection point). Of course the situation changes for different values of the beam radius.

## 5. TAYLOR EXPANSION OF DISPERSIVE PHASE

We perform a Taylor expansion of the dispersive phase

$$\Phi_{\text{disp}}(\omega) = kL \tag{S131}$$

$$= \frac{n(\omega)\omega L}{c}, \tag{S132}$$

analogous to Eq. (S16), and keep Taylor coefficients

$$b_{j,\text{disp}} = \left.\frac{\mathrm{d}^j \Phi_{\text{disp}}(\omega)}{\mathrm{d}\omega^j}\right|_{\omega=\omega_0} \tag{S133}$$

up to $j = 3$. The resulting parameters are available for many different optical materials [20]. Thus we find, for a material of thickness $L$, the change in the absolute phase

$$b_{0,\text{disp}} = \frac{\omega_0 L}{v_{\text{ph}}} \tag{S134}$$

with phase velocity

$$v_{\text{ph}} = \frac{c}{n_0} \tag{S135}$$

and the refractive index at center frequency

$$n_0 = n(\omega_0), \tag{S136}$$

the linear phase coefficient

$$b_{1,\text{disp}} = \frac{L}{v_{\text{gr}}} \tag{S137}$$

with group velocity

$$v_{\text{gr}} = \frac{c}{n_{\text{gr}}} \tag{S138}$$

and group index

$$n_{\text{gr}} = \left.\frac{\mathrm{d}k}{\mathrm{d}\omega}\right|_{\omega=\omega_0} \tag{S139}$$

defined via the frequency-dependent wave number $k$, the quadratic phase coefficient (or "group-delay dispersion")

$$b_{2,\text{disp}} = L\,\text{GVD} \tag{S140}$$

with group-velocity dispersion

$$\text{GVD} = \left.\frac{\mathrm{d}^2 k}{\mathrm{d}\omega^2}\right|_{\omega=\omega_0}, \tag{S141}$$

and the third-order phase coefficient

$$b_{3,\text{disp}} = L\,\text{TOD} \tag{S142}$$

with third-order dispersion

$$\text{TOD} = \left.\frac{\mathrm{d}^3 k}{\mathrm{d}\omega^3}\right|_{\omega=\omega_0}. \tag{S143}$$

## 6. ABSOLUTE AMPLITUDE SCALING OF SECOND-ORDER FIELDS

Here we derive a scaling factor for second-order generated fields ensuring that energy conservation can always be fulfilled. For this purpose we might envision a simple scaling procedure in which we calculate, in a first step, $E_\text{s}(t)$ with an arbitrary scaling, then obtain the pulse energy via Eq. (S40), and finally simply scale down $E_\text{s}(t)$ such that the pulse energy is only a user-provided fraction of the sum of input pulse energies. This would omit, however, the desired scaling with spatial and temporal pulse overlap that is an integral part of the present simulation model. For example, a second-harmonic signal increases with tighter focusing.

Thus, we need to define the proportionality factor between fundamental and second-order fields as an appropriate "global" constant that is not adjusted. If we still want to ensure that energy conservation and a maximal conversion efficiency are fulfilled for all possible situations, we have to calculate the maximum possible second-order field under optimal spatial–temporal conditions and use this result to scale all signals. Thus we ensure that in all other situations, the actual field will be smaller. Maximum nonlinear signal generation occurs with optimum spatial–temporal overlap (that we consider by calculating SHG of a single beam instead of SFG between two beams) at the highest possible peak intensity. The temporal intensity scales proportional to pulse energy according to Eq. (S43) and inversely proportional to the cross-section area according to Eq. (S44). Furthermore, it can be shown analytically that the highest possible SHG pulse energy is reached, for a given fundamental spectrum $A(\omega)$, if the spectral phase $\Phi(\omega)$ has zero curvature [21], i.e., a non-dispersed or "bandwidth-limited" pulse. Thus, we derive the scaling factor for the situation that the incident pulse has the "highest possible" pulse energy $W_\text{max}$, "smallest possible" beam radius $w_\text{min}$, and "shortest possible" pulse duration $\tau_\text{p,min}$. (The latter is strictly true for any given general spectral distribution $A(\omega)$ only if pulse duration is defined as a second-order moment, rather than as an intensity FWHM, but if we observe the condition to analyze a flat spectral phase, the result is correct in any event [21].)

Let us find $W_\text{max}$ first. Of course, laser pulses do not have an absolute upper bound of their energy. However, we need to analyze only the specific pulses generated with the chosen laser settings. Let us ignore the possibility for amplification of laser pulses once they are emitted by the laser. Amplification would change the subsequent analysis. In the absence of amplification, however, the pulse energy can only decrease due to absorption in samples, splitting of beams, imperfect optics, etc., such that we simply have $W_\text{max} = W_0$ according to Eq. (S42), where $W_0$ is the pulse energy of the laser-emitted pulse, and thus $S_\text{max} = S_0 = W_0$ in terms of the pulse-energy scaling factor (noting that the initial norm fulfills $E_0 = 1$).

The condition of a flat spectral phase for maximum SHG efficiency is reached, in our model calculation, by assuming the electric field profile of the pulse initially emitted by the laser (without dispersion) and quantified in Eq. (S47) in the case of a Gaussian.

Finally, the smallest beam radius is reached at the beam waist, $w_\text{min} = w_0$, for any given Gaussian beam. Thus we have to find the minimum possible beam waist that is fundamentally limited by diffraction. The half-divergence angle of a Gaussian beam, $\beta$, is defined via

$$\tan\beta = \frac{w(z)}{z} \tag{S144}$$

$$\xrightarrow[z \gg z_\text{R}]{} \frac{w_0}{z_\text{R}} \tag{S145}$$

$$= \frac{\lambda M^2}{\pi w_0}. \tag{S146}$$

Let us assume we cannot focus tighter than with a half-divergence angle of $\beta_\text{max} = 45^\circ$ so that $\tan\beta_\text{max} = 1$. Then we obtain

$$w_\text{min} = \frac{\lambda M^2}{\pi} \tag{S147}$$

for wavelength $\lambda$ and beam-quality factor $M^2$. Now we can calculate the maximum SHG pulse energy $W_{\mathrm{SHG,max}}$ under these optimal conditions and use it for appropriate scaling of SFG or SHG under any other condition. For this purpose, we first use Eq. (51) to determine

$$S_{\mathrm{SHG,max}} = S_{\mathrm{SFG,unscaled}} \tag{S148}$$

while setting

$$S_1 = S_2 = S_{\mathrm{max}} = S_0 = W_0, \tag{S149}$$

$$w_1(z) = w_2(z) = w_{\mathrm{min}} = \frac{\lambda M^2}{\pi}, \tag{S150}$$

$$x_1 = x_2, \tag{S151}$$

$$y_1 = y_2 \tag{S152}$$

with $m = 1$ in Eq. (51) from the main text (signifying second-harmonic generation) because we use the full power $W_0$ rather than splitting it first into two beams of half the energy each that are then overlapped again (which would give the identical result due to the squared response), so that

$$S_{\mathrm{SHG,max}} = \frac{\pi W_0^2}{\lambda^2 M^4\, \delta t}. \tag{S153}$$

Then, we obtain the norm $E_{\mathrm{SHG,max}}$, as defined in Eq. (S41), of the SHG envelope as defined in Eq. (49), using the $E$-normalized laser output pulse from Eq. (S47) for both envelopes $\tilde{E}_{1,t}(j_1) = \tilde{E}_{2,t}(j_2)$. From both quantities, the maximum (unscaled) SHG pulse energy is

$$W_{\mathrm{SHG,max}} = S_{\mathrm{SHG,max}} E^2_{\mathrm{SHG,max}} \tag{S154}$$

using Eq. (S40), which leads to Eq. (52) in the main text where we allow only a fraction $\eta_2$ of the fundamental pulse energy $W_0$ to be converted to SHG under optimum conditions.

## 7. DERIVATION OF NONLINEAR SIGNAL BEAM CURVATURE

Here we derive beam parameters of a signal beam arising from nonlinear response, i.e., in particular its beam radius and focus position, that can be used to obtain the complex beam parameter $q$. We follow, for the first steps, the treatment by Boyd [5], where it is shown that the Gaussian beam from Eq. (S31) can alternatively be written as

$$A(r,z) = \frac{A}{1+i\zeta} \exp\left[-\frac{r^2}{w_0^2(1+i\zeta)}\right] \tag{S155}$$

with the scaled longitudinal position parameter

$$\zeta = \frac{z}{z_{\mathrm{R}}}, \tag{S156}$$

at position $z$, measured with respect to the longitudinal position of the beam waist, the waist radius $w_0$, the Rayleigh length $z_{\mathrm{R}}$ from Eq. (S32), and an amplitude $A$ that we have set equal to 1 in Eq. (S31) because we considered the amplitude as part of the time- or frequency-dependent factors. Harmonic generation from a single incident beam is provided as a textbook example [5], but we here deviate from that treatment and instead consider the generalized case of $(n+1)$-wave mixing at nonlinear order $n$, arising from potentially distinct input beams. This can be described in the slowly varying amplitude approximation and in the paraxial approximation via the “paraxial wave equation”

$$2ik_{\mathrm{s}} \frac{\partial A_{\mathrm{s}}(r,z)}{\partial z} + \nabla_{\mathrm{T}}^2 A_{\mathrm{s}}(r,z) = -\frac{\omega_{\mathrm{s}}^2}{\varepsilon_0 c^2} P_{\mathrm{s}}(r,z) e^{i\Delta k z} \tag{S157}$$

with the transverse Laplace operator $\nabla_{\mathrm{T}}^2$ that is part of the full Laplace operator

$$\nabla^2 = \nabla_{\mathrm{T}}^2 + \frac{\partial^2}{\partial z^2}, \tag{S158}$$

while we ignore contributions $\partial^2 A/\partial z^2$ in Eq. (S157).

The nonlinear signal polarization

$$P_{\mathrm{s}}(r,z) = \varepsilon_0 \chi^{(n)}(\omega_{\mathrm{s}}, \omega_1, \dots, \omega_n) \prod_{i=1}^{n} A_i^{(*)}(r,z) \tag{S159}$$

is given in terms of the $n$th-order frequency-dependent nonlinear susceptibility $\chi^{(n)}$, evaluated at the signal frequency

$$\omega_{\mathrm{s}} = \sum_{i=1}^{n} \alpha_i \omega_i \tag{S160}$$

for incident center frequencies $\omega_i$, phase-matching coefficients $\alpha_i \in \{-1, +1\}$, and amplitudes

$$A_i^{(*)}(r,z) = \begin{cases} A_i(r,z), & \text{if } \alpha_i = +1, \\ A_i^*(r,z), & \text{if } \alpha_i = -1, \end{cases} \tag{S161}$$

such that complex conjugation (indicated by a star) is applied for those beams entering with a minus sign in the calculation of the phase mismatch

$$\Delta\mathbf{k} = \left( \sum_{i=1}^{n} \alpha_i \mathbf{k}_i \right) - \mathbf{k}_{\mathrm{s}} \tag{S162}$$

that in turn results from the incident wave vectors $\mathbf{k}_i$ and the signal wave vector $\mathbf{k}_{\mathrm{s}}$. In the case of perfect phase matching, $\Delta\mathbf{k} = 0$, one obtains, for the example of sum-frequency generation, $\mathbf{k}_{\mathrm{s}} = \mathbf{k}_1 + \mathbf{k}_2$.

Gaussian beams, written as Eq. (S155), solve the left-hand side of the paraxial wave equation in Eq. (S157) which can be shown by using the cylindrical coordinate representation for $\nabla_{\mathrm{T}}^2$, and thus a good ansatz for the signal beam is

$$A_{\mathrm{s}}(r,z) = \frac{A_{\mathrm{s}}(z)}{1 + i\zeta_{\mathrm{s}}} \exp\left[ -\frac{r^2}{w_{0,\mathrm{s}}^2 (1 + i\zeta_{\mathrm{s}})} \right] \tag{S163}$$

with the $z$-dependent amplitude function $A_{\mathrm{s}}(z)$ to allow taking into account the polarization source term on the right-hand side of the wave equation. Using Eq. (S163) in Eq. (S157), one arrives at an ordinary differential equation for $\mathrm{d}A_{\mathrm{s}}(z)/\mathrm{d}z$ that can be integrated directly to give the solution

$$\begin{aligned} A_{\mathrm{s}}(z) = \frac{i\omega_{\mathrm{s}}}{2c} \chi^{(n)}(\omega_{\mathrm{s}}, \omega_1, \dots, \omega_n) \int_{z-L/2}^{z+L/2} \frac{1 + i\zeta_{\mathrm{s}}'}{\prod_{i=1}^{n}(1 + i\alpha_i \zeta_i')} e^{i\Delta k z'} \\ \times \exp\left\{ -r^2 \left[ -\frac{1}{w_{0,\mathrm{s}}^2(1 + i\zeta_{\mathrm{s}})} + \sum_{i=1}^{n} \frac{1}{w_{0,i}^2 (1 + i\alpha_i \zeta_i)} \right] \right\} \mathrm{d}z', \end{aligned} \tag{S164}$$

where we are interested in the solution at position $z$ that we choose to be co-located with a sample of length $L$ because we want to obtain the correct transformation of beam parameters at the sample. We consider the limit of thin samples such that

$$\int_{z-L/2}^{z+L/2} f(z')\,\mathrm{d}z' \approx f(z)L. \tag{S165}$$

Since we want the solution to be represented as a Gaussian beam and the ansatz $A_{\mathrm{s}}(z)$ did not depend on $r$, the square-bracketed term in the $r$-containing exponent in the second line of Eq. (S164) has to be equal to 0, requiring

$$\frac{1}{w_{0,\mathrm{s}}^2 (1 + i\zeta_{\mathrm{s}})} = \sum_{i=1}^{n} \frac{1}{w_{0,i}^2 (1 + i\alpha_i \zeta_i)}. \tag{S166}$$

Making denominators real leads to

$$\frac{1 - i\zeta_{\mathrm{s}}}{w_{0,\mathrm{s}}^2 (1 + \zeta_{\mathrm{s}}^2)} = \sum_{i=1}^{n} \frac{1 - i\alpha_i \zeta_i}{w_{0,i}^2 (1 + \zeta_i^2)}. \tag{S167}$$

Comparing separately the real and imaginary parts leads to the conditions

$$\frac{1}{w_{0,\mathrm{s}}^2(1+\zeta_\mathrm{s}^2)} = \sum_{i=1}^{n} \frac{1}{w_{0,i}^2(1+\zeta_i^2)}, \tag{S168}$$

$$\frac{\zeta_\mathrm{s}}{w_{0,\mathrm{s}}^2(1+\zeta_\mathrm{s}^2)} = \sum_{i=1}^{n} \frac{\alpha_i \zeta_i}{w_{0,i}^2(1+\zeta_i^2)}. \tag{S169}$$

We note that

$$w(z) = w_0\sqrt{1+\zeta^2}, \tag{S170}$$

which is further discussed in Section 5.1 of the main paper, so that the condition in Eq. (S168) for the real part can be written as

$$\frac{1}{w_\mathrm{s}^2(z)} = \sum_{i=1}^{n} \frac{1}{w_i^2(z)}, \tag{S171}$$

which is the same result for the signal beam radius that we have already obtained by considering the purely two-dimensional Gaussian beam cross-section overlap in Section 2, Eq. (S79), where we had ignored beam curvature. We use this result to replace the denominator on the left-hand side of Eq. (S169), and Eq. (S170) to replace the denominator on the right-hand side, yielding

$$\zeta_\mathrm{s} = w_\mathrm{s}^2(z) \sum_{i=1}^{n} \frac{\alpha_i \zeta_i}{w_i^2(z)}. \tag{S172}$$

In the evaluation, we require the parameters $\zeta_i$ of the incident beams. From Eq. (S32), Eq. (S33), and Eq. (S34) we find that $z = \operatorname{Re} q$ (with respect to the beam-waist position) and $z_\mathrm{R} = -\operatorname{Im} q$. Using the definition for $\zeta$ in Eq. (S156), we obtain

$$\zeta = -\frac{\operatorname{Re} q}{\operatorname{Im} q} \tag{S173}$$

that can be inserted into the sum of Eq. (S172) for given incident beam parameters $q_i$. Lastly, the real-valued curvature radius $R(z)$ at position $z$, i.e., at the point of the thin sample, is given by

$$R(z) = z\left(1+\frac{1}{\zeta^2}\right) \tag{S174}$$

$$= \frac{\pi w_0^2}{\lambda}\left(\zeta + \frac{1}{\zeta}\right) \tag{S175}$$

$$= \frac{\pi w^2(z)}{\lambda(1+\zeta^2)} \frac{\zeta^2+1}{\zeta} \tag{S176}$$

$$= \frac{\pi w^2(z)}{\lambda \zeta}. \tag{S177}$$

Thus, the desired nonlinear signal Gaussian beam parameters are given by Eq. (S171), Eq. (S172), and Eq. (S177), from which the complex radius of curvature can be constructed.

## 8. OPTIMAL VERTEX DISTRIBUTION FOR GAUSSIAN BEAM MODELING

Optimal mesh spacing for the representation of three-dimensional objects has been discussed in the literature [22, 23]. We adapt that treatment for the specific situation of Gaussian laser beams. The main idea is to analyze the local "mesh curvature" and to require the distance between two neighboring mesh vertices to be inversely proportional to that curvature. In that way, for a mesh that is strongly curved locally, the mesh uses fine steps, and for a mesh that has small curvature, larger step sizes suffice because the rendering uses straight lines between mesh points.

Given the radial symmetry of the Gaussian beam, we analyze separately the curvature along and perpendicular to the direction of propagation, starting with the former. Assume we are given the relation

$$w(z) = w_0\sqrt{1+\left(\frac{z}{z_\mathrm{R}}\right)^2}, \tag{S178}$$

where we leave out the tilde signs of Eq. (61) for brevity and to indicate that the same treatment is applicable to any beam without necessarily making use of the mesh transformation of Eq. (74).

For analyzing the mesh curvature, we calculate the first and second derivatives of Eq. (S178) with respect to $z$ that read, respectively,

$$w'(z) = \frac{\mathrm{d}w(z)}{\mathrm{d}z} = w_0 \left[1 + \left(\frac{z}{z_\mathrm{R}}\right)^2\right]^{-\frac{1}{2}} \frac{z}{z_\mathrm{R}^2}, \tag{S179}$$

$$w''(z) = \frac{\mathrm{d}^2 w(z)}{\mathrm{d}z^2} = \frac{w_0}{z_\mathrm{R}^2} \left\{ \left[1 + \left(\frac{z}{z_\mathrm{R}}\right)^2\right]^{-\frac{1}{2}} - \left(\frac{z}{z_\mathrm{R}}\right)^2 \left[1 + \left(\frac{z}{z_\mathrm{R}}\right)^2\right]^{-\frac{3}{2}} \right\}. \tag{S180}$$

Let us evaluate $w''(z)$ at specific locations for illustration of the general behavior. At the origin, we find

$$w''(0) = \frac{w_0}{z_\mathrm{R}^2} \tag{S181}$$

which is the largest (longitudinal) mesh curvature along the whole beam, occurring at the beam waist. Note that the mesh curvature defined here is different from the curvature $R$ of the wave fronts, defined in Eq. (S33). The mesh curvature drops to

$$w''(z_\mathrm{R}) = \frac{\sqrt{2}}{4} w''(0) \approx 0.35\, w''(0) \tag{S182}$$

at the distance of one Rayleigh length, and

$$w''(z) \xrightarrow[x \to \infty]{} 0 \tag{S183}$$

as it should be, approaching the straight-line asymptote of the hyperbola of a Gaussian beam.

Following Eqs. (22) and (25) of Ref. [23] for $\theta \approx 0$, we obtain the local mesh step size

$$\Delta z(z) = \min \left\{ \frac{g(\varepsilon)}{|w''(z)|}, \Delta z_\mathrm{max} \right\} \tag{S184}$$

at local position $z$ along the propagation $\hat{\mathbf{z}}$ axis, with a user-provided maximal step size $\Delta z_\mathrm{max}$ that ensures a minimum number of mesh points for a certain distance, independent of the "optimal" number, and a function [22]

$$g(\varepsilon) \approx (1 - \varepsilon) \sqrt{40 \left(1 - \sqrt{1 - \frac{6}{5}\varepsilon}\right)} \tag{S185}$$

that depends on the desired tolerance $\varepsilon$ for the relative error of the approximated straight mesh segment compared to the real curved mesh segment. Exemplarily, requiring $\varepsilon = 1\ \%$, we get $g(\varepsilon) = 0.49$ for the scaling factor between inverse curvature and longitudinal mesh step size.

Now we calculate the total number of steps, $N_\mathrm{longitudinal}$, required to render a Gaussian beam along its longitudinal direction, by adding up the individual steps. Instead of a discrete sum, which would be correct, the corresponding approximate integral

$$N_\mathrm{longitudinal}(\varepsilon) \approx 2 \int_0^L \frac{\mathrm{d}z}{\Delta z(z)} \tag{S186}$$

for a laser segment ranging from $z = -L$ to $z = L$ (with the factor of 2 taking into account the mirror symmetry) allows obtaining a closed expression using Eq. (S179) and Eq. (S184), ignoring user-defined maximum step sizes,

$$N_\mathrm{longitudinal}(\varepsilon) = 2 \int_0^L \frac{w''(z)}{g(\varepsilon)} \mathrm{d}z \tag{S187}$$

$$= \frac{2}{g(\varepsilon)} \left[w'(L) - w'(0)\right] \tag{S188}$$

$$= \frac{2}{g(\varepsilon)} w_0 \left[1 + \left(\frac{L}{z_\mathrm{R}}\right)^2\right]^{-\frac{1}{2}} \frac{L}{z_\mathrm{R}^2}. \tag{S189}$$

The longer the beam, the more steps are required. In the limit of a long beam, $L \gg z_\mathrm{R}$, this can be simplified to

$$N_{\text{longitudinal,max}}(\varepsilon) = \frac{2w_0}{g(\varepsilon) z_\mathrm{R}} \tag{S190}$$

and, using the definition in Eq. (S32),

$$N_{\text{longitudinal,max}}(\varepsilon) = \frac{2\lambda M^2}{\pi g(\varepsilon) w_0}. \tag{S191}$$

This result is largest for a minimal $w_0$, i.e., a tight focus. Using the result for the minimal $w_0$ from Eqs. (S144)–(S147) in Eq. (S191), we obtain the very simple final result

$$N_{\text{longitudinal,max}}(\varepsilon) = \frac{2}{g(\varepsilon)}. \tag{S192}$$

For example, requiring again $\varepsilon = 1\,\%$, we need a maximum number of $N_{\text{longitudinal, max}}(1\,\%) = 4$ steps along the longitudinal direction, which can be rendered with 5 vertex points.

Next, we analyze the optimal mesh spacing along the circumference of the cross section. The curvature of a circle is given by the inverse of its radius, so that we obtain

$$y''(z) = \frac{\partial^2 y(x,z)}{\partial x^2} = \frac{1}{w(z)}, \tag{S193}$$

for a given radius $w(z)$ at position $z$, where we have chosen a coordinate system with arbitrary transverse $\hat{\mathbf{x}}$ and $\hat{\mathbf{y}}$ directions, because the result is in fact independent of the angular coordinate due to circular symmetry. Alternatively, one can derive and formulate the result using angular coordinates. Analogous to Eq. (S184), the mesh step size is then given by

$$\Delta x(z) = \frac{g(\varepsilon)}{|y''(z)|} = g(\varepsilon) w(z), \tag{S194}$$

with a total number of vertices along the circumference of length $2\pi w(z)$ of

$$N_{\text{circumference}}(\varepsilon) = \frac{2\pi w(z)}{\Delta x(z)} = \frac{2\pi}{g(\varepsilon)}, \tag{S195}$$

which is independent of $w(z)$ and thus independent of $z$. No matter what the size of the circle is, we should always use the same number of points. For example, requiring again $\varepsilon = 1\,\%$ and $g(\varepsilon) = 0.49$, we obtain

$$N_{\text{circumference}}(1\,\%) = 13. \tag{S196}$$

It is possible to arrive at the same result without making use of the approximations implicit in Eq. (S185). The chord length of a circle segment of angle $\phi$ is $2\sin(\phi/2)$, and thus the relative difference $\varepsilon$ between the two lengths is given by

$$1 - \varepsilon = \frac{2\sin\frac{\phi}{2}}{\phi}. \tag{S197}$$

For a given $\varepsilon = 1\,\%$, the numerical solution of Eq. (S197) delivers $N_{\text{circumference}}(1\,\%) = 12.8 \approx 13$ as above.

Combining Eq. (S192) and Eq. (S195), we arrive at a total number of

$$N_{\text{total,max}}(\varepsilon) = N_{\text{longitudinal,max}}(\varepsilon) N_{\text{circumference}}(\varepsilon) = \frac{4\pi}{g^2(\varepsilon)} \tag{S198}$$

and, at an error level of $1\,\%$, a maximum of $(4+1) \times 13 = 65$ vertices that suffice to describe any Gaussian laser beam, independent of its specific geometrical parameters [and $(6+1) \times 18 = 126$ for $\varepsilon = 0.5\,\%$]. If one desires to limit the absolute error instead of the relative error, the numeric results change, but the basic analysis above can still be used.

## 9. COLOR PERCEPTION OF A STANDARD OBSERVER

The human eye with normal vision contains three types of cone cells with different spectral sensitivities in the range of long (L), middle (M), and short (S) visible wavelengths. This trifold distribution forms the basis for being able to represent colors on display devices via additive mixing of three "primary colors" called red (R), green (G), and blue (B). We start by representing a color in the device-independent "Commission Internationale de l'Éclairage" (CIE) XYZ standard ("tristimulus values") in its most recent implementation [24] and employ the "2-deg XYZ color matching functions transformed from the CIE (2006) 2-deg LMS cone fundamentals," $\bar{x}(\lambda), \bar{y}(\lambda), \bar{z}(\lambda)$, sampled at a step size of 1 nm [25]. Given a laser spectral intensity $I(\lambda)$ (more accurately, "spectral radiance," but this is irrelevant due to the normalization discussed below), we obtain the CIE XYZ color coordinates as

$$X = \int_{\lambda_{\mathrm{min}}}^{\lambda_{\mathrm{max}}} \bar{x}(\lambda) I(\lambda)\, \mathrm{d}\lambda, \tag{S199}$$

$$Y = \int_{\lambda_{\mathrm{min}}}^{\lambda_{\mathrm{max}}} \bar{y}(\lambda) I(\lambda)\, \mathrm{d}\lambda, \tag{S200}$$

$$Z = \int_{\lambda_{\mathrm{min}}}^{\lambda_{\mathrm{max}}} \bar{z}(\lambda) I(\lambda)\, \mathrm{d}\lambda, \tag{S201}$$

by integration between $\lambda_{\mathrm{min}} = 390$ nm and $\lambda_{\mathrm{max}} = 830$ nm.

Moving to frequency-dependent fields and intensities, we transform the wavelength-dependent properties accordingly, using

$$\lambda(\omega) = \frac{2\pi c}{\omega} \tag{S202}$$

along with

$$\mathrm{d}\lambda = -\frac{2\pi c}{\omega^2} \mathrm{d}\omega, \tag{S203}$$

to make the transition

$$X = -\int_{\omega(\lambda_{\mathrm{min}})}^{\omega(\lambda_{\mathrm{max}})} \bar{x}[\lambda(\omega)] I(\omega) \frac{2\pi c}{\omega^2}\, \mathrm{d}\omega \tag{S204}$$

$$= 2\pi c \int_{\omega_{\mathrm{min}}}^{\omega_{\mathrm{max}}} \frac{\bar{x}[\lambda(\omega)]}{\omega^2} I(\omega)\, \mathrm{d}\omega \tag{S205}$$

$$\approx 2\pi c \sum_{j=0}^{N_{\mathrm{s}}-1} \bar{x}'_{\omega}(j) I_{\omega}(j)\, \delta\omega, \tag{S206}$$

where in the last line we adopt the discretized sampling from Eq. (S57) at frequency positions given by Eq. (S50) with indices $j = \{0, 1, \ldots, N_{\mathrm{s}} - 1\}$, frequency sampling step size as in Eq. (S51), number of samples $N_{\mathrm{s}}$, and minimum sampled frequency as in Eq. (S52). Here, the discretized color-matching functions are

$$\bar{x}'_{\omega}(j) = \begin{cases} \frac{\bar{x}[\lambda(\omega)]}{\omega^2}, & \text{if } \lambda_{\mathrm{min}} \leq \frac{2\pi c}{\omega} \leq \lambda_{\mathrm{max}}, \\ 0, & \text{otherwise}, \end{cases} \tag{S207}$$

wherein $\bar{x}[\lambda(\omega)]$ can be obtained from $\bar{x}(\lambda)$ by interpolative resampling onto the $\omega(j)$ grid using an intermediate spline fit.

Using our conventions, the (on-axis) spectral laser intensity $I_{\omega}(j)$ is defined with respect to spectral power $P(\omega)$ for a given beam radius $w$, which is in turn defined with respect to the complex spectral envelope $\tilde{E}_{\omega}(j)$ using a pulse-energy scaling factor $S$ as in Eq. (S56), so that together

$$I_{\omega}(j) = \frac{2S}{\pi w^2\, \delta\omega} \left| \tilde{E}_{\omega}(j) \right|^2 \tag{S208}$$

should be employed in Eq. (S206). Since the XYZ color coordinates will be normalized in Eqs. (S212)–(S214) anyway, we can omit some proportionality constants and define a modified coordinate

$$X' = \sum_{j=0}^{N_{\mathrm{s}}-1} \bar{x}'_{\omega}(j) \left| \tilde{E}_{\omega}(j) \right|^2 . \tag{S209}$$

Analogously, we obtain the (modified) coordinates

$$Y' = \sum_{j=0}^{N_s-1} \bar{y}'_\omega(j) \left|\tilde{E}_\omega(j)\right|^2, \tag{S210}$$

$$Z' = \sum_{j=0}^{N_s-1} \bar{z}'_\omega(j) \left|\tilde{E}_\omega(j)\right|^2, \tag{S211}$$

from which we obtain the chromaticity values,

$$x = \frac{X'}{X' + Y' + Z'}, \tag{S212}$$

$$y = \frac{Y'}{X' + Y' + Z'}, \tag{S213}$$

$$z = \frac{Z'}{X' + Y' + Z'}, \tag{S214}$$

that now lie in the interval [0, 1] each. Actually, the value pair $(x, y)$ alone is sufficient to define the color because $z$ can be obtained from the normalization condition as $z = 1 - x - y$. We will require $z$ for the next step.

Any RGB color can be transformed to a CIE representation using

$$\begin{pmatrix} x \\ y \\ z \end{pmatrix} = M \begin{pmatrix} R \\ G \\ B \end{pmatrix}, \tag{S215}$$

where $R$, $G$, and $B$ are linear RGB components (without gamma correction applied) and $M$ is a suitable transformation matrix that depends on the particular color space and thus should be chosen according to a specific device. Exemplarily, let us assume that the graphics device can represent colors according to the International Telecommunication Union (ITU) Recommendation BT.2020 standard (known as "Rec. 2020") that defines a wider gamut (i.e., representable color space) than the traditional RGB or sRGB standards. The RGB or sRGB standards can be implemented analogously, just using the respective differently defined values. According to published specifications, Rec. 2020 is characterized by the primary colors and the CIE D65 standard illuminant ("white point") in $(x, y)$ coordinates,

$$\text{Red: } (0.708,\ 0.292), \tag{S216}$$

$$\text{Green: } (0.170,\ 0.797), \tag{S217}$$

$$\text{Blue: } (0.131,\ 0.046), \tag{S218}$$

$$\text{White: } (0.3127,\ 0.3290). \tag{S219}$$

Using these values, one can construct $M$ and from that, its inverse $M^{-1}$, to obtain

$$\begin{pmatrix} R \\ G \\ B \end{pmatrix}_{\text{unbounded}} = M^{-1} \begin{pmatrix} x \\ y \\ z \end{pmatrix}, \tag{S220}$$

with values for $M^{-1}$ in the case of Rec. 2020 given by

$$M^{-1} = \begin{pmatrix} 1.7166512 & -0.3556708 & -0.2533663 \\ -0.6666844 & 1.6164812 & 0.0157685 \\ 0.0176399 & -0.0427706 & 0.9421031 \end{pmatrix}. \tag{S221}$$

Note that any of the recovered RGB values may lie outside of the allowed [0, 1] interval if a given CIE color cannot be represented in the RGB system of the chosen color space, i.e., in our case if

the color is outside the Rec. 2020 gamut. We arrive at the bounded (linear) RGB coordinates by clamping, if required,

$$R = \max\{0, \min[R_{\text{unbounded}}, 1]\}, \tag{S222}$$

$$G = \max\{0, \min[G_{\text{unbounded}}, 1]\}, \tag{S223}$$

$$B = \max\{0, \min[B_{\text{unbounded}}, 1]\}. \tag{S224}$$

Now we have obtained the correct color but still want to render an appropriate luminance. For this purpose, we employ the "alpha" (A) channel in the RGBA system that represents opacity, where $A = 1$ means completely opaque and $A = 0$ completely transparent. Thus, if we want to represent a "laser spot" that has high luminance scattered off a surface, we desire a high value for $A$ such that the material of the underlying scattering object in essence does not shine through, and for a low-intensity spot we desire a low $A$ such that the laser-beam scattering is barely visible and the underlying material is visible. The CIE XYZ standard is defined such that the Y channel corresponds to luminance (taking into account human perception according to the "standard observer"), sometimes also called the xyY color space, i.e., taking $Y$ together with the chromaticity values $x$ and $y$ from Eq. (S212) and Eq. (S213), respectively. Above, we defined modified coordinates $X'Y'Z'$ in which $Y'$ takes already into account the spectral shape but not yet the absolute intensity in terms of pulse energy and beam radius. We obtain the desired $Y$ by re-introducing the correct scaling factors,

$$Y = 4c\frac{S}{w^2}Y'. \tag{S225}$$

Again, we employ a useful normalization such that we can ignore the constant factor $4c$ and define

$$A = \min\left[1, \frac{\frac{S}{w^2}Y'}{A_0}\right] \tag{S226}$$

with the reference

$$A_0 = \frac{S_0}{w_0^2}Y_0' \tag{S227}$$

obtained under the conditions for which maximum opacity shall be reached. If under any conditions, one obtains $\frac{S}{w^2}Y' > A_0$, the color cannot increase the perceived luminance, i.e., the intensity is "saturated." While one may wish to avoid such a scenario and define $A_0$ as the achievable maximum under any conditions, this may make it difficult to see any laser spot under other, less intense, conditions, depending on the pulse energy, spectral range, and beam radius of the laser, and the dynamic range of the display device. Thus, it may be appropriate to introduce a gamma correction for the alpha channel to create a rendering that covers a range large enough to observe the laser spot under a variety of conditions.

## 10. FEATURES AND LIMITATIONS

We summarize in Table S2 basic features and consequences of the physical model of the present work. This list is not meant to be exhaustive but rather to capture essential points for a quick overview. All individual entries are discussed in more detail in other sections and in the main text.

**Table S2.** Features and limitations of physical model.

| Property | Choice | Consequence |
|---|---|---|
| Beam profile | Gaussian | Finite beam overlap included |
| Beam quality | $M^2$ factor | Real beam divergence approximated |
| Beam symmetry | Radially symmetric | No astigmatism |
| Beam clipping | Diffraction-free | Geometrical effects included; no gratings |
| Polarization direction | Scalar electric fields | No birefringence; no polarization |
| Pulse shape | Discrete samples | Numerical calculation of modulations |
| First-order response | Response function | Dispersion and absorption included |
| Second-order response | Instantaneous | Pulse-shape effects included |

## REFERENCES

1. M. V. Klein and T. E. Furtak, *Optics* (Wiley, Hoboken, 1986), 2nd ed.
2. M. Born and E. Wolf, *Principles of Optics: Electromagnetic Theory of Propagation, Interference and Diffraction of Light* (Cambridge University Press, Cambridge, 1999), 7th ed.
3. W. Zinth and U. Zinth, *Optik. Lichtstrahlen – Wellen – Photonen* (Oldenbourg Wissenschaftsverlag, München, 2005).
4. L. Novotny and B. Hecht, *Principles of Nano-Optics* (Cambridge University Press, Cambridge, 2012), 2nd ed.
5. R. W. Boyd, *Nonlinear Optics* (Academic Press, Burlington, 2008), 3rd ed.
6. B. E. A. Saleh and M. C. Teich, *Fundamentals of Photonics* (Wiley, Hoboken, 2019), 3rd ed.
7. S. Mukamel, *Principles of Nonlinear Optical Spectroscopy* (Oxford University Press, New York, 1995), 1st ed.
8. J.-C. Diels and W. Rudolph, *Ultrashort Laser Pulse Phenomena: Fundamentals, Techniques, and Applications on a Femtosecond Time Scale* (Academic Press Inc, Amsterdam, 2006), 2nd ed.
9. R. Trebino, *Frequency-Resolved Optical Gating: The Measurement of Ultrashort Laser Pulses* (Springer, New York, 2002), 1st ed.
10. M. Wollenhaupt, A. Assion, and T. Baumert, "Femtosecond laser pulses: Linear properties, manipulation, generation and measurement," in *Springer Handbook of Lasers and Optics,* F. Träger, ed. (Springer Science+Business Media, New York, 2007), pp. 937–983.
11. A. M. Weiner, *Ultrafast Optics* (John Wiley & Sons Inc., Hoboken, 2009), 1st ed.
12. M. Cho, *Two-Dimensional Optical Spectroscopy* (CRC Press, Boca Raton, 2009).
13. P. Hamm and M. Zanni, *Concepts and Methods of 2D Infrared Spectroscopy* (Cambridge University Press, New York, 2011), 1st ed.
14. L. Valkunas, D. Abramavicius, and T. Mančal, *Molecular Excitation Dynamics and Relaxation* (Wiley-VCH, Weinheim, 2013), 1st ed.
15. J. Yuen-Zhou, J. J. Krich, I. Kassal, *et al.*, *Ultrafast Spectroscopy* (IOP Publishing, Bristol, 2014), 1st ed.
16. J. Alda, "Laser and Gaussian beam propagation and transformation," in *Encyclopedia of Optical Engineering,* C. Hoffman and R. Driggers, eds. (CRC Press, Boca Raton, 2003), pp. 999–1013, 2nd ed.
17. S. Akturk, X. Gu, P. Gabolde, and R. Trebino, "The general theory of first-order spatio-temporal distortions of Gaussian pulses and beams," Opt. Express **13**, 8642–8661 (2005).
18. H. Kogelnik, "Imaging of optical modes – Resonators with internal lenses," Bell. Sys. Tech. J. **44**, 455–494 (1965).
19. H. Kogelnik, "On the propagation of Gaussian beams of light through lenslike media including those with a loss or gain variation," Appl. Opt. **4**, 1562–1569 (1965).
20. M. N. Polyanskiy, "Refractive index database," https://refractiveindex.info. Accessed Jan. 8, 2021.
21. T. Brixner, "Adaptive femtosecond quantum control," Ph.D. thesis, Universität Würzburg (2001).
22. R. J. Cass, S. E. Benzley, R. J. Meyers, and T. D. Blacker, "Generalized 3-D paving: An

automated quadrilateral surface mesh generation algorithm," Int. J. Numer. Meth. Engng **39**, 1475–1489 (1996).
23. C. K. Lee, "On curvature element-size control in metric surface mesh generation," Int. J. Numer. Meth. Engng **50**, 787–807 (2001).
24. A. Stockman, "Cone fundamentals and CIE standards," Curr. Opin. Behav. Sci. **30**, 87–93 (2019).
25. "Colour & Vision Research Laboratory," http://www.cvrl.org. Accessed Jan 28, 2025.
